# Supplementary material for: Robust Precoding for FDD MISO Systems via Minorization Maximization
Source: arXiv:2411.02615 source file (2024-11-04)
Supplement: Supplementary file 1 [file Appendix.tex]

%We start by defining the matrix $\bs{X}=\bs{Z}+\bs{T}^\HH\bs{U}\bs{T}$. The objective of \eqref{eq:AWAMSEmin3} can therefore be written as
%\begin{equation} \label{eq:objDelta}
%    \begin{aligned}
%    &\tr(\bs{U})  - 2 \Re\{\tr (\bs{A}(\delta)^{-1}\bs{T}^\HH \bs{U}\bs{U}\bs{T}) \}\\
%       &+\tr (\bs{A}(\delta)^{-1}\bs{T}^\HH \bs{U}\bs{U} \bs{T} \bs{A}(\delta)^{-1} \bs{X}) \\      &+ \frac{1}{P_\tdl}\tr(\bs{A}(\delta)^{-2}\bs{T}^\HH \bs{U}\bs{U} \bs{T}) \tr (\bs{U}\bs{G}\bs{G}^\ast) - \log_2(\det(\bs{U}))
 %   \end{aligned}
%\end{equation}
The first derivative of \eqref{eq:AWAMSEmin3} w.r.t. $\delta$ reads as
\begin{equation}
    \begin{aligned}
    \frac{\partial}{\partial \delta}&=2\tr(\bs{A}^{-1}\bs{T}^\HH \bs{U}\bs{U}\bs{T} \bs{A}^{-1})-2\tr(\bs{B}^{-1}\bs{A}^{-1}\bs{T}^\HH \bs{U}\bs{U}\bs{T} \bs{A}^{-1})\\
    &-2\frac{1}{P_\tdl} \tr(\bs{A}^{-2}\bs{T}^\HH \bs{U}\bs{U}\bs{T} \bs{A}^{-1})\tr (\bs{U}\bs{G}\bs{G}^\ast)
    \end{aligned}
\end{equation}
where $\bs{B}^{-1}=\bs{A}^{-1}\bs{X}=(\bs{I}+\delta\bs{X}^{-1})^{-1}$ and $\bs{X}=\bs{Z}+\bs{T}^\HH\bs{U}\bs{T}$. From the matrix inversion lemma, it follows that $\bs{I}-\bs{B}^{-1}=\delta \bs{A}^{-1}$. The derivative can, therefore be rewritten as
\begin{equation}
    \begin{aligned}
    \frac{\partial}{\partial \delta}&=2\tr(\bs{A}^{-2}\bs{T}^\HH \bs{U}\bs{U}\bs{T} \bs{A}^{-1}) \left(\delta -\frac{\tr (\bs{U}\bs{G}\bs{G}^\ast)}{P_\tdl}\right)\overset{!}{=} 0
    \end{aligned}
\end{equation}
and the optimal $\delta^\text{opt}$ is hence given by \eqref{eq:DeltaOpt}.
